# Supplementary material for: The partonic structure of the electron at the next-to-leading logarithmic accuracy in QED
Source: arXiv:1911.12040 ancillary file (2022-07-25)
Supplement: Supplementary file 1 [file recursive.pdf]

**The partonic structure of the electron at the next-to-leading logarithmic accuracy in QED**

V. Bertone, M. Cacciari, S. Frixione, G. Stagnitto

We report here explicit expressions for the $\hat{J}_k^{\rm LL}(z)$ and $\hat{J}_k^{\rm NLL}(z)$ functions which appear in eq. (A.5) and (A.6) of the paper. Accordingly to eq. (A.7), these terms vanish in the $z \to 1$ limit. Results are reported for the non-singlet, singlet and photon PDFs.

As indicated in Appendix A, the terms $\hat{J}_2^{\rm NLL}(z)$ receive some contributions that we have computed only numerically. We report here only the analytical part. The final result for $\hat{J}_2^{\rm NLL}(z)$ is then given by the sum of $\hat{J}_{2,{\rm an}}^{\rm NLL}(z)$, the function reported here, and $\hat{J}_{2,{\rm num}}^{\rm NLL}(z)$, the contribution calculated numerically.

* * * * * * * * * * * * * * * * * * * * * * *

$$\hat{J}^{\rm LL}_{\rm NS,0} = 1 - z$$

$$\hat{J}^{\rm LL}_{\rm NS,1} = \frac{1}{z-1} \times \Bigg( 3z^2 \log(z) + (1-z)(z+3) - 4(z-1)^2 \log(1-z) + \log(z) \Bigg)$$

$$\hat{J}^{\rm LL}_{\rm NS,2} = \frac{1}{4(z-1)} \times \Bigg( -24\Big(z^2-1\Big)\mathrm{Li}_2(z) + 24\Big(-z^2+2\Big(z^2+1\Big)\log(z)+3\Big)\log(1-z) - 2\log(z)\Big(-9z^2+7z^2\log(z)+ \log(z)-3\Big) + (z-1)\Big(4\pi^2(3z-1)-3(5z+19)\Big) - 48(z-1)^2\log^2(1-z) - 48z(\log(2-2z)-\log(2z)) \Bigg)$$

$$\hat{J}^{\rm NLL}_{\rm NS,0} = (1-z)(L_0 - 2\log(1-z) - 1)$$

$$\hat{J}^{\rm NLL}_{\rm NS,1} = \frac{1}{18b_0(z-1)(z+1)} \times \Bigg( 36\pi b_0^2 L_0 z^3 - 36\pi b_0^2 L_0 z^2 - 36\pi b_0^2 L_0 z + 36\pi b_0^2 L_0 - 36\pi b_0^2 z^3 - 72\pi b_0^2 z^3 \log(1-z) + 36\pi b_0^2 z^2 + 72\pi b_0^2 z^2 \log(1-z) + 36\pi b_0^2 z + 72\pi b_0^2 z \log(1-z) - 72\pi b_0^2 \log(1-z) - 36\pi b_0^2 - 18b_0 L_0 z^3 - 72b_0 L_0 z^3 \log(1-z) + 54b_0 L_0 z^3 \log(z) - 54b_0 L_0 z^2 + 72b_0 L_0 z^2 \log(1-z) + 54b_0 L_0 z^2 \log(z) + 18b_0 L_0 z + 72b_0 L_0 z \log(1-z) + 18b_0 L_0 z \log(z) - 72b_0 L_0 \log(1-z) + 18b_0 L_0 \log(z) + 54b_0 L_0 + 44b_0 N_F z^3 + 12b_0 N_F z^3 \log(z) - 68b_0 N_F z^2 + 12b_0 N_F z^2 \log(z) - 44b_0 N_F z + 12b_0 N_F z \log(z) + 12b_0 N_F \log(z) + 68b_0 N_F + 72b_0\Big(z^3 - z^2 - 2z + 2\Big)\mathrm{Li}_2(-z) + 216b_0 z \mathrm{Li}_2\Big(\frac{1}{z+1}\Big) - 36b_0(z-1)(z+1)^2\mathrm{Li}_2(1-z) - 216b_0\mathrm{Li}_2\Big(\frac{1}{z+1}\Big) + 153b_0 z^3 - 6\pi^2 b_0 z^3 + 108b_0 z^3 \log^2(1-z) - 27b_0 z^3 \log^2(z) + 54b_0 z^3 \log(1-z) - 90b_0 z^3 \log(z) - 72b_0 z^3 \log(1-z)\log(z) + 72b_0 z^3 \log(z)\log(z+1) - 135b_0 z^2 + 6\pi^2 b_0 z^2 - 108b_0 z^2 \log^2(1-z) + 9b_0 z^2 \log^2(z) + 18b_0 z^2 \log(1-z) - 90b_0 z^2 \log(z) - 72b_0 z^2 \log(1-z)\log(z) - 72b_0 z^2 \log(z)\log(z+1) - 153b_0 z - 18\pi^2 b_0 z - 108b_0 z \log^2(1-z) - 9b_0 z \log^2(z) + 108b_0 z \log^2(z+1) + 108b_0 \log^2(1-z) + 27b_0 \log^2(z) - 108b_0 \log^2(z+1) - 54b_0 z \log(1-z) + 72b_0 z \log(z) - 144b_0 z \log(z)\log(z+1) - 18b_0 \log(1-z) + 72b_0 \log(z) + 144b_0 \log(z)\log(z+1) + 135b_0 + 18\pi^2 b_0 + 36\pi b_1 z^3 - 36\pi b_1 z^2 - 36\pi b_1 z + 36\pi b_1 \Bigg)$$

$$\hat{J}^{\rm NLL}_{\rm NS,2,an} = \frac{1}{36b_0 z\Big(z^2-1\Big)} \times \Bigg( (1-z)z\Big(144(L_0-1)\pi^2\Big(z^2-1\Big)b_0^3 - 8\pi\Big(18L_0(z+1)(z+3) - 2N_F(z+1)(11z-17) + 3\Big(3\Big(-8+\pi^2\Big)z^2 - 15z + \pi^2 + 9\Big)\Big)b_0^2 + \Big(2\Big(-2N_F\Big(4\pi^2(z-1) - 19z + 63\Big)(z+1) + 9(57z-73)(z+1) + 6\pi^2\Big(z(17z+3) + 12b_1\Big(z^2-1\Big) - 2\Big)\Big) - 9L_0(z+1)\Big(8\pi^2(z-1) - 3(5z+19)\Big)\Big)b_0 - 144b_1\pi(z+1)(z+3)\Big) + 2\Big(6b_0\log^3(z)z^4 - 18b_0\log^2(z)z^4 - 63b_0 L_0 \log^2(z)z^4 - 36b_0 N_F \log^2(z)z^4 + 54b_0^2\pi\log^2(z)z^4 -$$

$216b_0^2\pi(\log(1-z)-\log(z))z^4-342b_0\log(z)z^4+81b_0L_0\log(z)z^4-156b_0N_F\log(z)z^4+$

$72b_0\log^2(2)\log(z)z^4-72b_0\log(2)\log(z)z^4-18b_0\pi^2\log(z)z^4-216b_1\pi\log(z)z^4-216b_0^2L_0\pi\log(z)z^4-$

$24b_0^2N_F\pi\log(z)z^4+18b_0\log^3(z)z^3+144b_0\log^2(z)z^3-63b_0L_0\log^2(z)z^3-36b_0N_F\log^2(z)z^3-$

$18b_0^2\pi\log^2(z)z^3+234b_0\log(z)z^3+297b_0L_0\log(z)z^3-12b_0N_F\log(z)z^3-72b_0\log^2(2)\log(z)z^3+$

$144b_0\log(2)\log(z)z^3+42b_0\pi^2\log(z)z^3+288b_0^2\pi\log(z)z^3-216b_1\pi\log(z)z^3-216b_0^2L_0\pi\log(z)z^3-$

$24b_0^2N_F\pi\log(z)z^3-6b_0\log^3(z)z^2+54b_0\log^2(z)z^2-9b_0L_0\log^2(z)z^2-12b_0N_F\log^2(z)z^2+$

$18b_0^2\pi\log^2(z)z^2+306b_0\log(z)z^2+243b_0L_0\log(z)z^2+68b_0N_F\log(z)z^2-72b_0\log^2(2)\log(z)z^2+$

$288b_0\log(2)\log(z)z^2+66b_0\pi^2\log(z)z^2-36b_0^2\pi\log(z)z^2-72b_1\pi\log(z)z^2-72b_0^2L_0\pi\log(z)z^2-$

$24b_0^2N_F\pi\log(z)z^2+288b_0(z-1)^2(z+1)\log^3(1-z)z-18b_0\log^3(z)z-48b_0(z-4)(z-1)(z+4)\log^3(z+1)z-$

$144b_0\log^2(z)z-9b_0L_0\log^2(z)z-12b_0N_F\log^2(z)z-54b_0^2\pi\log^2(z)z-270b_0\log(z)z+27b_0L_0\log(z)z-$

$76b_0N_F\log(z)z+72b_0\log^2(2)\log(z)z-144b_0\log(2)\log(z)z-42b_0\pi^2\log(z)z-108b_0^2\pi\log(z)z-$

$72b_1\pi\log(z)z-72b_0^2L_0\pi\log(z)z-24b_0^2N_F\pi\log(z)z-36b_0(z+1)\log^2(1-z)\Big((6L_0(z-1)+12b_0\pi(z-1)-$

$5z-7)(z-1)+\Big(11z^2+1\Big)\log(z)\Big)z+\log(1-z)\Big(144\pi^2(z-1)^2(z+1)b_0^3+72\pi\Big(4L_0(z+1)(z-1)^2-3z(z-1)+$

$3\Big)b_0^2-(z-1)\Big(108L_0(z+1)(z+3)+32N_F((3-8z)z+11)+3\Big(-27z(7z+4)+4\pi^2\Big(9z^2+z-6\Big)+120\log^2(2)+$

$81\Big)\Big)b_0+12\Big(3(z-1)(z(2z+5)+1)\log^2(z)+(z+1)\Big((30\pi b_0+27L_0+4N_F-30)z^2-24z+9L_0+4N_F+$

$6b_0\pi+27\Big)\log(z)+24(z-1)(2\log(2)-\log(z))\log(z+1)\Big)b_0+288b_1\pi(z-1)^2(z+1)\Big)z-108b_0\log^2(z)-$

$18b_0\Big(-16\log(2)z^4+8(\log(z)+2\log(2))z^3+4(15z-13)\log(z)z+8(z-1)(\log(1-z)+\log(z)+2\log(2))z+$

$(z-1)(z(12\pi b_0+z(14z+29)-23)-12)\Big)\log^2(z+1)+12b_0\log(2)\Big(-4\pi^2z\Big(z^3+2z-1\Big)+(z-1)(z+$

$1)(z(9z+7)+3)\log(8)+2z\Big(z\Big(4z^2+z+16\Big)-11\Big)\log^2(2)\Big)-216b_0\log(2)\log(z)-12b_0\Big(6z(z+1)(z(2z-$

$3)+2)\log^2(z)+6(z-1)z\Big(-4z+2b_0\pi\Big(z^2-2\Big)-3\Big)\log(z)+(z-1)\Big(12z\log^2(2)\Big(z^2+4\Big)+\pi^2\Big(z^3+z\Big)+$

$6\Big(z\Big((-1+2\log(2))z^2+z+5\Big)-2z(\log(1-z)+\log(2))+3\Big)(\log(z)+\log(2))\Big)\Big)\log(z+1)\Big)+18b_0\Big(-$

$16z(z+1)\mathrm{Li}_3\Big(\frac{1-z}{2}\Big)(z-1)^2+16z(z+1)\mathrm{Li}_3\Big(\frac{z-1}{2z}\Big)(z-1)^2-56z(z+1)\mathrm{Li}_3\Big(\frac{z}{z+1}\Big)(z-1)^2+16z(z+$

$$1)\mathrm{Li}_3\left(\frac{2z}{z+1}\right)(z-1)^2-16z\Big((\log(z+1)-\log(1-z))z^2+\log(1-z)-\log(z+1)-5\log(2)\Big)\mathrm{Li}_2\left(\frac{1-z}{2}\right)(z-1)+8z(z+1)(7z+4)\mathrm{Li}_3(1-z)(z-1)+4z(z+1)(7z+5)\mathrm{Li}_3(z)(z-1)-16z\left(z^2+4\right)\mathrm{Li}_3\left(\frac{z+1}{2}\right)(z-1)+4z(z+1)\Big((4\pi b_0+3L_0-8)z^2+2(z(-8\log(1-z)+\log(z)+2\log(z+1))-4(\log(z+1)-\log(1-z)))z-3L_0+\log\left((z-1)^8\right)-2\log(z)+4\log(z+1)-4b_0\pi+11\Big)\mathrm{Li}_2(1-z)+8\left(z^2-1\right)(z(2\log(2)(z-1)-z+2)-2(z-1)z\log(1-z)+3)\mathrm{Li}_2\left(\frac{z-1}{2z}\right)-4\Big((z-1)\Big(z\Big(z(15z-1)+4b_0\pi\left(z^2-2\right)-20\Big)-6\Big)+4z\Big(\log(z)z^3+\log(1-z)z-\log(1-z)+\log(z)+(z(z+6)-5)\log(z+1)\Big)\Big)\mathrm{Li}_2(-z)+8z\Big((z-1)\left(4z^2-2z+6\log(1-z)-6b_0\pi-3\right)+2\left(z^3+5z-4\right)\log(z+1)\Big)\mathrm{Li}_2\left(\frac{1}{z+1}\right)-4\left(z^2-1\right)(z(5z-8)+10(z-1)z\log(z+1)-6)\mathrm{Li}_2\left(\frac{z}{z+1}\right)+8\left(z^2-1\right)(z(2\log(2)(z-1)-z+2)-2(z-1)z\log(z+1)+3)\mathrm{Li}_2\left(\frac{2}{z+1}-1\right)-8z^2\left(z^2-1\right)\mathrm{Li}_3\left(\frac{z-1}{z}\right)-8z(z+1)(z(7z-16)+7)\mathrm{Li}_3(-z)+16z\left(-3z^3+z^2+z-3\right)\mathrm{Li}_3\left(\frac{1}{z+1}\right)+z(z(z(61z-69)+59)+29)\zeta(3)\Big)\Big)$$

$$\hat{J}^{\text{LL}}_{\text{S},0} = 1 - z$$

$$\hat{J}^{\text{LL}}_{\text{S},1} = \frac{\Big((4N_F+3)z^2 - 4N_F + 1\Big)\log(z)}{z-1} - \frac{2N_F(z-1)(z(4z+7)+4)}{3z} - z - 4(z-1)\log(1-z) - 3$$

$$\hat{J}^{\text{LL}}_{\text{S},2} = -\frac{1}{36(z-1)z} \times \Bigg( -64N_F^2z^4 + 16N_F^2z^3 + 96N_F^2z^3\log(z) + 96N_F^2z^2 + 16N_F^2z - 96N_F^2z\log(z) - 64N_F^2 +$$
$$72(8N_F+3)\Big(z^2-1\Big)z\mathrm{Li}_2(z) - 384N_Fz^4\log(z) - 552N_Fz^3 - 96\pi^2N_Fz^3 + 144N_Fz^3\log^2(z) +$$
$$96N_Fz^3\log(z) + 1104N_Fz^2 + 288N_Fz^2\log(z) + 24\log(1-z)\Big((z-1)\Big(4N_F\Big(4z^3+3z^2-3z-4\Big) +$$
$$9z(z+3)\Big) - 18\Big(z^3+z\Big)\log(z)\Big) - 552N_Fz + 96\pi^2N_Fz - 144N_Fz\log^2(z) - 108\pi^2z^3 + 135z^3 +$$
$$126z^3\log^2(z) - 162z^3\log(z) + 144\pi^2z^2 + 378z^2 - 432z^2\log(z) - 36\pi^2z - 513z + 432(z-1)^2z\log^2(1-$$
$$z) + 18z\log^2(z) - 54z\log(z)\Bigg)$$

$$\hat{J}^{\text{NLL}}_{\text{S},0} = L_0(1-z) + z - 2(1-z)\log(1-z) - 1$$

$$\hat{J}^{\text{NLL}}_{\text{S},1} = -\frac{1}{18b_0(z-1)z(z+1)} \times \Bigg(72b_0N_Fz^5 + 48b_0L_0N_Fz^5 - 96b_0N_F\log(z)z^5 - 108b_0\log^2(1-z)z^4 -$$
$$9b_0\log^2(z)z^4 + 108b_0N_F\log^2(z)z^4 - 9b_0z^4 + 18b_0L_0z^4 - 296b_0N_Fz^4 + 36b_0L_0N_Fz^4 - 54b_0\log(1-$$
$$z)z^4 + 72b_0L_0\log(1-z)z^4 + 72b_0^2\pi\log(1-z)z^4 + 18b_0\log(z)z^4 - 54b_0L_0\log(z)z^4 - 48b_0N_F\log(z)z^4 -$$
$$72b_0L_0N_F\log(z)z^4 + 72b_0\log(1-z)\log(z)z^4 + 72b_0\log(z)\log(z+1)z^4 + 18b_0\pi^2z^4 + 36b_0^2\pi z^4 -$$
$$36b_1\pi z^4 - 36b_0^2L_0\pi z^4 + 108b_0\log^2(1-z)z^3 + 27b_0\log^2(z)z^3 + 108b_0N_F\log^2(z)z^3 - 9b_0z^3 +$$
$$54b_0L_0z^3 + 104b_0N_Fz^3 - 84b_0L_0N_Fz^3 - 18b_0\log(1-z)z^3 - 72b_0L_0\log(1-z)z^3 - 72b_0^2\pi\log(1-$$
$$z)z^3 + 18b_0\log(z)z^3 - 54b_0L_0\log(z)z^3 + 264b_0N_F\log(z)z^3 - 72b_0L_0N_F\log(z)z^3 + 72b_0\log(1-$$
$$z)\log(z)z^3 - 72b_0\log(z)\log(z+1)z^3 - 18b_0\pi^2z^3 - 36b_0^2\pi z^3 + 36b_1\pi z^3 + 36b_0^2L_0\pi z^3 + 108b_0\log^2(1-$$
$$z)z^2 - 27b_0\log^2(z)z^2 - 108b_0N_F\log^2(z)z^2 + 108b_0\log^2(z+1)z^2 + 9b_0z^2 - 18b_0L_0z^2 + 368b_0N_Fz^2 -$$
$$84b_0L_0N_Fz^2 + 54b_0\log(1-z)z^2 - 72b_0L_0\log(1-z)z^2 - 72b_0^2\pi\log(1-z)z^2 - 18b_0L_0\log(z)z^2 +$$
$$120b_0N_F\log(z)z^2 + 72b_0L_0N_F\log(z)z^2 - 144b_0\log(z)\log(z+1)z^2 + 216b_0\mathrm{Li}_2\Big(\frac{1}{z+1}\Big)z^2 - 42b_0\pi^2z^2 -$$
$$36b_0^2\pi z^2 + 36b_1\pi z^2 + 36b_0^2L_0\pi z^2 - 108b_0\log^2(1-z)z + 9b_0\log^2(z)z - 108b_0N_F\log^2(z)z -$$

$$108b_0\log^2(z+1)z+9b_0z-54b_0L_0z-176b_0N_Fz+36b_0L_0N_Fz+18b_0\log(1-z)z+72b_0L_0\log(1-z)z+72b_0^2\pi\log(1-z)z-18b_0L_0\log(z)z-192b_0N_F\log(z)z+72b_0L_0N_F\log(z)z+144b_0\log(z)\log(z+1)z+36b_0(z-1)(z+1)^2\mathrm{Li}_2(1-z)z+72b_0\left(z^3-z^2-2z+2\right)\mathrm{Li}_2(-z)z-216b_0\mathrm{Li}_2\left(\frac{1}{z+1}\right)z+42b_0\pi^2z+36b_0^2\pi z-36b_1\pi z-36b_0^2L_0\pi z-72b_0N_F+48b_0L_0N_F-96b_0N_F\log(z)\Bigg)$$

$$\hat{J}^{\mathrm{NLL}}_{\mathrm{S},2,\mathrm{an}}=\frac{1}{108b_0z\left(z^2-1\right)}\times\Bigg(608b_0N_F^2z^5+192b_0L_0N_F^2z^5-432b_0N_Fz^5+96b_0N_F\pi^2z^5-960b_0^2N_F\pi z^5+1152b_1N_F\pi z^5+1152b_0^2L_0N_F\pi z^5+144b_0N_F^2z^4+144b_0L_0N_F^2z^4-486b_0z^4-405b_0L_0z^4-3852b_0N_Fz^4+1656b_0L_0N_Fz^4+360b_0^2\pi^3z^4+432b_0^3\pi^2z^4+324b_0\pi^2z^4-432b_0b_1\pi^2z^4-432b_0^3L_0\pi^2z^4+216b_0L_0\pi^2z^4+120b_0N_F\pi^2z^4+432b_1\pi z^4+432b_0^2L_0\pi z^4-3984b_0^2N_F\pi z^4+864b_1N_F\pi z^4+864b_0^2L_0N_F\pi z^4-1328b_0N_F^2z^3-336b_0L_0N_F^2z^3+1350b_0z^3-1539b_0L_0z^3+4092b_0N_Fz^3-1656b_0L_0N_Fz^3-360b_0^2\pi^3z^3-432b_0^3\pi^2z^3-504b_0\pi^2z^3+432b_0b_1\pi^2z^3+432b_0^3L_0\pi^2z^3-216b_0L_0\pi^2z^3-216b_0N_F\pi^2z^3-1080b_0^2\pi z^3+1296b_1\pi z^3+1296b_0^2L_0\pi z^3+3504b_0^2N_F\pi z^3-2016b_1N_F\pi z^3-2016b_0^2L_0N_F\pi z^3-176b_0N_F^2z^2-336b_0L_0N_F^2z^2+486b_0z^2+405b_0L_0z^2+5004b_0N_Fz^2-1656b_0L_0N_Fz^2-648b_0^2\pi^3z^2-432b_0^3\pi^2z^2+108b_0\pi^2z^2+432b_0b_1\pi^2z^2+432b_0^3L_0\pi^2z^2-216b_0L_0\pi^2z^2-216b_0N_F\pi^2z^2-432b_1\pi z^2-432b_0^2L_0\pi z^2+6672b_0^2N_F\pi z^2-2016b_1N_F\pi z^2-2016b_0^2L_0N_F\pi z^2+720b_0N_F^2z+144b_0L_0N_F^2z-1350b_0z+1539b_0L_0z-3660b_0N_Fz+1656b_0L_0N_Fz+864b_0(z-1)\left((\log(z+1)-\log(1-z))z^2+\log(1-z)-\log(z+1)-5\log(2)\right)\mathrm{Li}_2\left(\frac{1-z}{2}\right)z-144b_0\left(z\left(4z^2+z+16\right)-11\right)\log^3(2)z+288b_0\pi^2\left(z^3+2z-1\right)\log(2)z+648b_0^2\pi^3z+432b_0^3\pi^2z+72b_0\pi^2z-432b_0b_1\pi^2z-432b_0^3L_0\pi^2z+216b_0L_0\pi^2z+120b_0N_F\pi^2z+1080b_0^2\pi z-1296b_1\pi z-1296b_0^2L_0\pi z-2544b_0^2N_F\pi z+864b_1N_F\pi z+864b_0^2L_0N_F\pi z+32b_0N_F^2+192b_0L_0N_F^2-1152b_0N_F+96b_0N_F\left(4(-3L_0+N_F-4)z^5-9L_0z^4+4N_F\right)(\log(1-z)-\log(z))+6\Big(288b_0(z-1)^2z(z+1)\log^3(1-z)-12b_0(z+1)\Big((1-z)(3z(12\pi b_0+6L_0-6(2\pi b_0+L_0)z+5z+7)+2N_F(z-1)(z(4z+7)+4))+3\left((4N_F+11)z^3-4N_Fz+z\right)\log(z)\Big)\log^2(1-z)+\Big(144\pi^2(z-1)^2z(z+1)b_0^3+72\pi z\left(z^2-1\right)(4L_0(z-1)-3(z+1))b_0^2+\Big(16(z-3)z(z+1)(3z-1)N_F^2+4(12L_0(z(7z(z+1)-3)-4)+z(z(z(229z-117)-237)+181)+8)N_F-3(z-$$

$$1)z(36L_0(z+1)(z+3)+\pi^2(44z^2-4z-56)+3((z-36)z-40\log^2(2)-37)))b_0+12(-3(z-$$

$$1)z(-z(2z+5)+2N_F(2z^2+z-1)-5)\log^2(z)+(-8N_F^2(z-1)z(z+1)^2+2N_F(z(8z^3-9(z+2)z+$$

$$12L_0(z^2-1)+15)+8)(z+1)+3z(-z(10z+7)+3L_0(z+1)(3z^2+1)+2b_0\pi(z+1)(5z^2+1)+$$

$$1))\log(z)+24(z-1)z(\log(z)-\log(4))\log(z+1))b_0+288b_1\pi(z-1)^2z(z+1))\log(1-z)+6b_0z(z^2-$$

$$1)(5z+12N_F(z+2)-1)\log^3(z)+3b_0\log^2(z)(z(16N_F^2(z-1)(z+1)^2-3L_0((8N_F+7)z^2-8N_F+$$

$$1)(z+1)+4N_F(-20z^3+(8z+15)z+30b_0\pi(z^2-1)-7)(z+1)+6(-b_0\pi(z-1)^3+z(z(7z-8)-13)+$$

$$4))+24z(z+1)(z(2z-3)+2)\log(z+1)+36)-\log(z)(12\pi(z+1)(3z(-2z(z+1)+L_0(6z^2+2)-$$

$$1)+4N_F(z(4(z-3)z(z+1)+6L_0(z^2-1)+9)+8))b_0^2+(3L_0z(16N_F^2(z-1)(z+1)^2-9(z(3z+8)+$$

$$1)(z+1)+16N_Fz(4z+3))+2z(8(z+1)(z(16z-13)-7)N_F^2+2(18\pi^2(z-1)(z+1)(z+2)+z(z(105z-$$

$$152)-83)+238)N_F+3\pi^2(z((5-9z)z+9)-13)+9(z+1)(4\log^2(2)(z-1)^2+8\log(2)(z-1)-z^2+$$

$$3)+144z\log(2))-216\log(2))b_0+72z\log(z+1)((1-z)(-4z+2b_0\pi(z^2-2)-3)+(13-15z)\log(z+$$

$$1))b_0+72b_1\pi z(z+1)((4N_F+3)z^2-4N_F+1))+6b_0(12\log(z)(-\log(1-z)-\log(z+1)+\log(2))z^4+$$

$$\log(z+1)(2z(\pi^2(z-1)(z^2+1)+(2(z-1)(z^2+4)\log(2)-z^3)\log(64))+12(2(z-1)\log(2)z^3+$$

$$2(z(z+2)-1)z-2(z-1)(\log(1-z)+\log(2))z-3)(\log(z)+\log(2))+\log(z+1)(-48\log(2)z^4+$$

$$24(\log(z)+2\log(2))z^3+8(z-1)(3(\log(1-z)+\log(z)+2\log(2))+(z^2-16)\log(z+1))z+3(z-$$

$$1)(z(12\pi b_0+z(14z+29)-23)-12)))))+18b_0(4(z+1)(-8z(z^2-1)N_F^2+4(z-1)(6L_0z(z+1)+(z-$$

$$3)z(2z+3)-2)N_F+3z(3L_0(z^2-1)+4b_0\pi(z^2-1)+3)+6z(8\log(1-z)+4N_F(\log(1-z)-\log(z))-$$

$$\log(z)-2\log(z+1)+z(-4(N_F+1)z\log(1-z)+(z-2N_F(z-3))\log(z)-2z\log(z+1)+4(\log(z+1)-$$

$$\log(1-z)))))\mathrm{Li}_2(1-z)+3(16z(z+1)\mathrm{Li}_3(\frac{1-z}{2})(z-1)^2-16z(z+1)\mathrm{Li}_3(\frac{z-1}{2z})(z-1)^2+56z(z+$$

$$1)\mathrm{Li}_3(\frac{z}{z+1})(z-1)^2-16z(z+1)\mathrm{Li}_3(\frac{2z}{z+1})(z-1)^2+8(z+1)(z(-2\log(2)z+z+2\log(2)-2)+2(z-$$

$$1)z\log(z+1)-3)\mathrm{Li}_2(\frac{2}{z+1}-1)(z-1)+16z(z^2+4)\mathrm{Li}_3(\frac{z+1}{2})(z-1)-8(z^2-1)(z(2\log(2)(z-$$

$$1)-z+2)-2(z-1)z\log(1-z)+3)\mathrm{Li}_2(\frac{z-1}{2z})+4((z-1)(z(z(15z-1)+4b_0\pi(z^2-2)-20)-6)+$$

$$4z\Big(\log(z)z^3+\log(1-z)z-\log(1-z)+\log(z)+(z(z+6)-5)\log(z+1)\Big)\Big)\mathrm{Li}_2(-z)+8z\Big((z-1)\Big(-$$

$$4z^2+2z-6\log(1-z)+6b_0\pi+3\Big)-2\Big(z^3+5z-4\Big)\log(z+1)\Big)\mathrm{Li}_2\left(\frac{1}{z+1}\right)+4\Big(z^2-1\Big)(z(5z-8)+$$

$$10(z-1)z\log(z+1)-6)\mathrm{Li}_2\left(\frac{z}{z+1}\right)+8z\Big(z^2-1\Big)(3z+4N_F(z+1)+8)\mathrm{Li}_3(1-z)-8z(6N_F+z)\Big(z^2-$$

$$1\Big)\mathrm{Li}_3\left(\frac{z-1}{z}\right)+8z(z+1)(z(7z-16)+7)\mathrm{Li}_3(-z)+4z(8zN_F+20N_F+3z+9)\Big(z^2-1\Big)\mathrm{Li}_3(z)+16z(z+$$

$$1)(z(3z-4)+3)\mathrm{Li}_3\left(\frac{1}{z+1}\right)-z(16N_F(z-1)(z+1)(2z+5)+z(z(21z+67)+99)-107)\zeta(3)\Big)\Big)-$$

$$216b_0(z-1)(z+1)(z(9z+7)+3)\log^2(2)+96b_0N_F\pi^2-2688b_0^2N_F\pi+1152b_1N_F\pi+1152b_0^2L_0N_F\pi\Bigg)$$

$$\hat{J}^{\text{LL}}_{\gamma,0} = \frac{(1-z)^2}{z} + \frac{1-z}{z}$$

$$\hat{J}^{\text{LL}}_{\gamma,1} = -\frac{1}{6z} \times \left( (z-1)(4N_F(z-2)+3z) - 12\left(z^2-3z+2\right)\log(1-z) + 6(z-2)z\log(z) \right)$$

$$\hat{J}^{\text{LL}}_{\gamma,2} = \frac{1}{36}\Big(16N_F^2 z + \frac{32N_F^2}{z} - 48N_F^2 + 64N_F z^2 - \frac{24\log(1-z)\left((z-1)(2N_F(z-2)+3z)+6\left(z^2-2z+2\right)\log(z)\right)}{z} - 636N_F z - \frac{496N_F}{z} - 72N_F z\log^2(z) + 144N_F\log^2(z) + 240N_F z\log(z) - \frac{192N_F\log(z)}{z} - 48N_F\log(z) + 1068N_F - \frac{288\text{Li}_2(z)}{z} + \frac{144\left(z^2-3z+2\right)\log^2(1-z)}{z} - 24\pi^2 z + 99z + 18z\log^2(z) - 36\log^2(z) + 72z\log(z) - 180\log(z) + 72\pi^2 - 99\Big)$$

$$\hat{J}^{\text{NLL}}_{\gamma,0} = \frac{(L_0-1)\left(z^2-3z+2\right) - 2\left(z^2-2z+2\right)\log(z)}{z}$$

$$\hat{J}^{\text{NLL}}_{\gamma,1} = -\frac{2\pi b_1 z}{b_0} - \frac{4\pi b_1}{b_0 z} + \frac{6\pi b_1}{b_0} - 2\pi b_0 L_0 z - \frac{4\pi b_0 L_0}{z} + 6\pi b_0 L_0 + 2\pi b_0 z + \frac{4\pi b_0}{z} + 4\pi b_0 z\log(z) + \frac{8\pi b_0\log(z)}{z} - 8\pi b_0\log(z) - 6\pi b_0 - \frac{2L_0 N_F z}{3} - \frac{4L_0 N_F}{3z} + \frac{\log(1-z)((z-1)(6L_0(z-2) - 4N_F z + 8N_F - 9z + 12) + 6(z-2)z\log(z))}{3z} + 2L_0 N_F - \frac{L_0 z}{2} + 2L_0\log(z) - L_0 z\log(z) + \frac{L_0}{2} - \frac{26N_F z}{9} - \frac{28N_F}{9z} - \frac{8}{3}N_F\log(z) + \frac{4}{3}N_F z\log(z) + \frac{8N_F\log(z)}{3z} + 6N_F + 2(z-2)\text{Li}_2(1-z) - \frac{3\left(z^2-3z+2\right)\log^2(1-z)}{z} - \frac{5z}{2} + \frac{1}{2}z\log^2(z) - \log^2(z) + \frac{5}{2}z\log(z) + \frac{5}{2}\Big)$$

$$\hat{J}^{\text{NLL}}_{\gamma,2,\text{an}} = \frac{1}{216 b_0 z\left(z^2-1\right)} \times \Big( 448b_0N_F z^5 + 384b_0L_0N_F z^5 - 768b_0N_F\log(z)z^5 - 1296b_0\log^3(1-z)z^4 + 360b_0\log^3(z)z^4 + 576b_0N_F\log^3(z)z^4 + 1872b_0\log^3(z+1)z^4 + 416b_0N_F^2 z^4 + 96b_0L_0N_F^2 z^4 - 972b_0\log^2(1-z)z^4 + 864b_0L_0\log^2(1-z)z^4 - 144b_0N_F\log^2(1-z)z^4 + 2160b_0^2\pi\log^2(1-z)z^4 + 432b_0\log^2(z)z^4 + 108b_0L_0\log^2(z)z^4 - 864b_0N_F\log^2(z)z^4 - 432b_0L_0N_F\log^2(z)z^4 - 1296b_0\log(1-z)\log^2(z)z^4 - 216b_0^2\pi\log^2(z)z^4 - 648b_0\log^2(z+1)z^4 + 837b_0z^4 + 594b_0L_0z^4 + 14148b_0N_F z^4 - 3816b_0L_0N_F z^4 + 192b_0N_F^2\log(2-2z)z^4 - 432b_0L_0\log(2-2z)z^4 - 2484b_0\log(1-z)z^4 - 1440b_0N_F\log(1-z)z^4 - 288b_0L_0N_F\log(1-z)z^4 + 432b_0\pi^2\log(1-z)z^4 + 432b_0^2\pi\log(1-z)z^4 - 1728b_1\pi\log(1-z)z^4 - 1728b_0^2L_0\pi\log(1-z)z^4 + 576b_0^2N_F\pi\log(1-z)z^4 + 1512b_0\log^2(1-$$

$z)\log(z)z^4+702b_0\log(z)z^4-1080b_0N_F\log(z)z^4+1440b_0L_0N_F\log(z)z^4+648b_0\log(1-z)\log(z)z^4-$

$864b_0L_0\log(1-z)\log(z)z^4-1728b_0^2\pi\log(1-z)\log(z)z^4-1728b_0^3\pi^2\log(z)z^4+288b_0\pi^2\log(z)z^4-$

$648b_0^2\pi\log(z)z^4+864b_1\pi\log(z)z^4+864b_0^2L_0\pi\log(z)z^4-1152b_0^2N_F\pi\log(z)z^4-192b_0N_F^2\log(2z)z^4+$

$432b_0L_0\log(2z)z^4-432b_0\log^2(z)\log(z+1)z^4-864b_0\log(z)\log(z+1)z^4-864b_0\text{Li}_2\left(\frac{1}{z+1}\right)z^4+$

$864b_0\log(z+1)\text{Li}_2\left(\frac{1}{z+1}\right)z^4-432b_0\text{Li}_2\left(\frac{z}{z+1}\right)z^4+3456b_0\log(z+1)\text{Li}_2\left(\frac{z}{z+1}\right)z^4-3024b_0\text{Li}_3(1-$

$z)z^4-1728b_0\text{Li}_3\left(\frac{z-1}{z}\right)z^4-3888b_0\text{Li}_3(z)z^4+216b_0\text{Li}_3\left(z^2\right)z^4+1728b_0\text{Li}_3\left(\frac{z}{z+1}\right)z^4+864b_0\zeta(3)z^4-$

$864b_0^3\pi^2z^4+180b_0\pi^2z^4+864b_0b_1\pi^2z^4+864b_0^3L_0\pi^2z^4-144b_0L_0\pi^2z^4+48b_0N_F\pi^2z^4+648b_0^2\pi z^4+$

$432b_1\pi z^4+432b_0^2L_0\pi z^4+960b_0^2N_F\pi z^4+576b_1N_F\pi z^4+576b_0^2L_0N_F\pi z^4+3024b_0\log^3(1-z)z^3-$

$432b_0\log^3(z)z^3-1152b_0N_F\log^3(z)z^3+288b_0\log^3(z+1)z^3-864b_0N_F^2z^3-288b_0L_0N_F^2z^3+2700b_0\log^2(1-$

$z)z^3-2592b_0L_0\log^2(1-z)z^3+432b_0N_F\log^2(1-z)z^3-6480b_0^2\pi\log^2(1-z)z^3+432b_0\log^2(z)z^3-$

$216b_0L_0\log^2(z)z^3-1728b_0N_F\log^2(z)z^3+864b_0L_0N_F\log^2(z)z^3+4320b_0\log(1-z)\log^2(z)z^3+$

$432b_0^2\pi\log^2(z)z^3-3456b_0\log^2(z+1)z^3-1728b_0\log(z)\log^2(z+1)z^3-3645b_0z^3-594b_0L_0z^3-$

$12868b_0N_Fz^3+6024b_0L_0N_Fz^3-576b_0N_F^2\log(1-z)z^3+3564b_0\log(1-z)z^3+432b_0L_0\log(1-z)z^3+$

$3744b_0N_F\log(1-z)z^3+864b_0L_0N_F\log(1-z)z^3-1008b_0\pi^2\log(1-z)z^3-1296b_0^2\pi\log(1-z)z^3+$

$5184b_1\pi\log(1-z)z^3+5184b_0^2L_0\pi\log(1-z)z^3-1728b_0^2N_F\pi\log(1-z)z^3+384b_0N_F^2\log(z)z^3-$

$3024b_0\log^2(1-z)\log(z)z^3+2916b_0\log(z)z^3-1080b_0L_0\log(z)z^3-17520b_0N_F\log(z)z^3-$

$288b_0L_0N_F\log(z)z^3+1296b_0\log(1-z)\log(z)z^3+1728b_0L_0\log(1-z)\log(z)z^3+3456b_0^2\pi\log(1-$

$z)\log(z)z^3+3456b_0^3\pi^2\log(z)z^3-864b_0\pi^2\log(z)z^3+864b_0^2\pi\log(z)z^3-1728b_1\pi\log(z)z^3-$

$1728b_0^2L_0\pi\log(z)z^3+2304b_0^2N_F\pi\log(z)z^3-864b_0\log^2(z)\log(z+1)z^3-3456b_0\log(z)\log(z+1)z^3-$

$576b_0\pi^2\log(z+1)z^3-864b_0\text{Li}_2\left(\frac{1}{z+1}\right)z^3+1728b_0\log(z+1)\text{Li}_2\left(\frac{1}{z+1}\right)z^3-6048b_0\text{Li}_2\left(\frac{z}{z+1}\right)z^3-$

$3456b_0\log(z+1)\text{Li}_2\left(\frac{z}{z+1}\right)z^3+7776b_0\text{Li}_3(1-z)z^3+3456b_0\text{Li}_3\left(\frac{z-1}{z}\right)z^3+7776b_0\text{Li}_3(z)z^3+$

$432b_0\text{Li}_3\left(z^2\right)z^3-3456b_0\text{Li}_3\left(\frac{z}{z+1}\right)z^3-6048b_0\zeta(3)z^3-2016b_0\log^3(2)z^3+864b_0\pi^2\log(2)z^3+$

$2592b_0^3\pi^2z^3 - 468b_0\pi^2z^3 - 2592b_0b_1\pi^2z^3 - 2592b_0^3L_0\pi^2z^3 + 432b_0L_0\pi^2z^3 - 144b_0N_F\pi^2z^3 - 648b_0^2\pi z^3 -$

$432b_1\pi z^3 - 432b_0^2L_0\pi z^3 - 1728b_0^2N_F\pi z^3 - 1728b_1N_F\pi z^3 - 1728b_0^2L_0N_F\pi z^3 - 432b_0\log^3(1-z)z^2 -$

$936b_0\log^3(z)z^2 - 576b_0N_F\log^3(z)z^2 + 3888b_0\log^3(z+1)z^2 + 32b_0N_F^2z^2 + 96b_0L_0N_F^2z^2 - 756b_0\log^2(1-$

$z)z^2 + 864b_0L_0\log^2(1-z)z^2 - 144b_0N_F\log^2(1-z)z^2 + 2160b_0^2\pi\log^2(1-z)z^2 - 432b_0\log^2(z)z^2 -$

$108b_0L_0\log^2(z)z^2 + 2016b_0N_F\log^2(z)z^2 + 432b_0L_0N_F\log^2(z)z^2 + 3024b_0\log(1-z)\log^2(z)z^2 +$

$216b_0^2\pi\log^2(z)z^2 - 648b_0\log^2(z+1)z^2 - 9504b_0\log(z)\log^2(z+1)z^2 + 1971b_0z^2 - 594b_0L_0z^2 -$

$16324b_0N_Fz^2 + 840b_0L_0N_Fz^2 + 192b_0N_F^2\log(2-2z)z^2 + 432b_0L_0\log(2-2z)z^2 + 1404b_0\log(1-$

$z)z^2 - 864b_0N_F\log(1-z)z^2 - 288b_0L_0N_F\log(1-z)z^2 + 144b_0\pi^2\log(1-z)z^2 + 432b_0^2\pi\log(1-z)z^2 -$

$1728b_1\pi\log(1-z)z^2 - 1728b_0^2L_0\pi\log(1-z)z^2 + 576b_0^2N_F\pi\log(1-z)z^2 - 1512b_0\log^2(1-z)\log(z)z^2 -$

$702b_0\log(z)z^2 + 3960b_0N_F\log(z)z^2 - 2592b_0L_0N_F\log(z)z^2 - 648b_0\log(1-z)\log(z)z^2 + 864b_0L_0\log(1-$

$z)\log(z)z^2 + 1728b_0^2\pi\log(1-z)\log(z)z^2 - 1728b_0^3\pi^2\log(z)z^2 - 864b_0\pi^2\log(z)z^2 + 648b_0^2\pi\log(z)z^2 -$

$864b_1\pi\log(z)z^2 - 864b_0^2L_0\pi\log(z)z^2 - 1152b_0^2N_F\pi\log(z)z^2 - 192b_0N_F^2\log(2z)z^2 - 432b_0L_0\log(2z)z^2 -$

$432b_0\log^2(z)\log(z+1)z^2 - 864b_0\log(z)\log(z+1)z^2 - 2016b_0\pi^2\log(z+1)z^2 + 7776b_0\log(z+$

$1)\mathrm{Li}_2\left(\frac{1}{z+1}\right)z^2 - 1296b_0\mathrm{Li}_2\left(\frac{z}{z+1}\right)z^2 - 1728b_0\log(z)\mathrm{Li}_2\left(\frac{z}{z+1}\right)z^2 - 3456b_0\log(z+1)\mathrm{Li}_2\left(\frac{z}{z+1}\right)z^2 +$

$6480b_0\mathrm{Li}_3(1-z)z^2 + 5184b_0\mathrm{Li}_3\left(\frac{z-1}{z}\right)z^2 + 5616b_0\mathrm{Li}_3(z)z^2 + 216b_0\mathrm{Li}_3\left(z^2\right)z^2 - 1728b_0\mathrm{Li}_3\left(\frac{z}{z+1}\right)z^2 -$

$864b_0\zeta(3)z^2 - 864b_0^3\pi^2z^2 - 180b_0\pi^2z^2 + 864b_0b_1\pi^2z^2 + 864b_0^3L_0\pi^2z^2 - 144b_0L_0\pi^2z^2 + 48b_0N_F\pi^2z^2 -$

$648b_0^2\pi z^2 - 432b_1\pi z^2 - 432b_0^2L_0\pi z^2 - 192b_0^2N_F\pi z^2 + 576b_1N_F\pi z^2 + 576b_0^2L_0N_F\pi z^2 - 3024b_0\log^3(1-z)z -$

$144b_0\log^3(z)z + 1152b_0N_F\log^3(z)z - 4608b_0\log^3(z+1)z + 864b_0N_F^2z + 288b_0L_0N_F^2z - 2700b_0\log^2(1-$

$z)z + 2592b_0L_0\log^2(1-z)z - 432b_0N_F\log^2(1-z)z + 6480b_0^2\pi\log^2(1-z)z - 432b_0\log^2(z)z +$

$216b_0L_0\log^2(z)z + 1728b_0N_F\log^2(z)z - 864b_0L_0N_F\log^2(z)z - 2592b_0\log(1-z)\log^2(z)z -$

$432b_0^2\pi\log^2(z)z + 3456b_0\log^2(z+1)z + 10368b_0\log(z)\log^2(z+1)z + 3645b_0z + 594b_0L_0z + 12420b_0N_Fz -$

$6408b_0L_0N_Fz + 576b_0N_F^2\log(1-z)z - 3564b_0\log(1-z)z - 432b_0L_0\log(1-z)z - 3744b_0N_F\log(1-$

$$z)z - 864b_0L_0N_F\log(1-z)z + 1008b_0\pi^2\log(1-z)z + 1296b_0^2\pi\log(1-z)z - 5184b_1\pi\log(1-z)z -$$

$$5184b_0^2L_0\pi\log(1-z)z + 1728b_0^2N_F\pi\log(1-z)z - 384b_0N_F^2\log(z)z + 3024b_0\log^2(1-z)\log(z)z -$$

$$2916b_0\log(z)z + 1080b_0L_0\log(z)z + 18288b_0N_F\log(z)z + 288b_0L_0N_F\log(z)z - 1296b_0\log(1-z)\log(z)z -$$

$$1728b_0L_0\log(1-z)\log(z)z - 3456b_0^2\pi\log(1-z)\log(z)z - 3456b_0^3\pi^2\log(z)z + 288b_0\pi^2\log(z)z -$$

$$864b_0^2\pi\log(z)z + 1728b_1\pi\log(z)z + 1728b_0^2L_0\pi\log(z)z - 2304b_0^2N_F\pi\log(z)z + 864b_0\log^2(z)\log(z+1)z +$$

$$2592b_0\log(z)\log(z+1)z + 2016b_0\pi^2\log(z+1)z + 1728b_0\text{Li}_2\left(\frac{1}{z+1}\right)z - 10368b_0\log(z+1)\text{Li}_2\left(\frac{1}{z+1}\right)z +$$

$$5184b_0\text{Li}_2\left(\frac{z}{z+1}\right)z + 3456b_0\log(z+1)\text{Li}_2\left(\frac{z}{z+1}\right)z - 4320b_0\text{Li}_3(1-z)z - 4320b_0\text{Li}_3(z)z -$$

$$432b_0\text{Li}_3\left(z^2\right)z + 3456b_0\text{Li}_3\left(\frac{z}{z+1}\right)z + 2592b_0\zeta(3)z + 2016b_0\log^3(2)z - 864b_0\pi^2\log(2)z - 2592b_0^3\pi^2z +$$

$$324b_0\pi^2z + 2592b_0b_1\pi^2z + 2592b_0^3L_0\pi^2z - 432b_0L_0\pi^2z + 144b_0N_F\pi^2z + 648b_0^2\pi z + 432b_1\pi z + 432b_0^2L_0\pi z +$$

$$1728b_0^2N_F\pi z + 1728b_1N_F\pi z + 1728b_0^2L_0N_F\pi z + 1728b_0\log^3(1-z) - 1440b_0\log^3(z+1) - 448b_0N_F^2 -$$

$$192b_0L_0N_F^2 + 1728b_0\log^2(1-z) - 1728b_0L_0\log^2(1-z) + 288b_0N_F\log^2(1-z) - 4320b_0^2\pi\log^2(1-z) -$$

$$1152b_0N_F\log^2(z) + 1296b_0\log^2(z+1) + 864b_0\log(z)\log^2(z+1) - 2808b_0 + 2176b_0N_F + 2976b_0L_0N_F -$$

$$384b_0N_F^2\log(2-2z) + 1080b_0\log(1-z) + 2304b_0N_F\log(1-z) + 576b_0L_0N_F\log(1-z) - 576b_0\pi^2\log(1-z) -$$

$$864b_0^2\pi\log(1-z) + 3456b_1\pi\log(1-z) + 3456b_0^2L_0\pi\log(1-z) - 1152b_0^2N_F\pi\log(1-z) - 2880b_0N_F\log(z) +$$

$$1152b_0L_0N_F\log(z) + 3456b_0^3\pi^2\log(z) + 2304b_0^2N_F\pi\log(z) + 384b_0N_F^2\log(2z) + 864b_0\log^2(z)\log(z+1) +$$

$$2592b_0\log(z)\log(z+1) + 576b_0\pi^2\log(z+1) - 144b_0\left(z^2-1\right)\Big(2N_Fz^2 + 12b_0\pi z^2 + 6z^2 - 4N_Fz + 3(z-$$

$$6)\log(z)z - 24b_0\pi z - 15z - 12L_0 + 4N_F + \left(-9z^2 + 18z + 12\right)\log(1-z) + 12\Big)\text{Li}_2(1-z) + 432b_0(z-1)\Big(-$$

$$3z^3 - 25z^2 + 2\left(3z^2 + z - 12\right)\log(z+1)z - 30z - 8(z+1)^2\log(z) - 12\Big)\text{Li}_2(-z) + 2592b_0\text{Li}_2\left(\frac{z}{z+1}\right) +$$

$$1728b_0\log(z)\text{Li}_2\left(\frac{z}{z+1}\right) + 1728b_0\text{Li}_3(z) - 432b_0\text{Li}_3\left(z^2\right) - 3456b_0\zeta(3) + 1728b_0^3\pi^2 + 144b_0\pi^2 -$$

$$1728b_0b_1\pi^2 - 1728b_0^3L_0\pi^2 + 288b_0L_0\pi^2 - 96b_0N_F\pi^2 - 768b_0^2N_F\pi - 1152b_1N_F\pi - 1152b_0^2L_0N_F\pi\Bigg)$$
